# Supplementary material for: Kernel KMeans clustering splits for end-to-end unsupervised decision trees
Source: arXiv:2402.12232 source file (2024-02-19)
Supplement: Supplementary file 1 [file extended_benchmark.tex]

%We first give the WAES scores of the previously described benchmark in Table.~\ref{tab:benchmark_small_wad}. We can observe that while Kauri is not always better than the KMeans+Tree baseline, it still manages to provide a reasonable tree structure with low WAES scores. It does not beat the shallowest related work ExShallow or IMM except on the car dataset, yet seems competitive enough with ExKMC. The reason for which IMM, ExShallow and RDM display better performances is simply the harshest constraints on the tree depth because theses methods seek as many leaves as clusters, limiting thus strongly the number of rules to find and lowering the WAES in exchange for worst clustering performances as seen in the previous section. To further investigate some differences, we observe in Fig.~\ref{fig:mice_digits} the differences in WAES scores between KMeans+Tree, Kauri and ExKMC. We did not put the other methods due to their number of leaves restrictions. We observe that overall, for a fixed amount of leaves to use, we obtained explanations with lower WAES scores than ExKMC while maintaining an ARI that is close to KMeans+Tree.%We did not put ExShallow because its float hyperparameter for depth control did not offer exact control over the number of leaves. 
