# Supplementary material for: Kernel KMeans clustering splits for end-to-end unsupervised decision trees
Source: arXiv:2402.12232 source file (2024-02-19)
Supplement: Supplementary file 2 [file model_selection.tex]

\begin{figure}
    \centering
    \subfloat[][Iris (2/2/11)]{\includegraphics[width=0.2\linewidth]{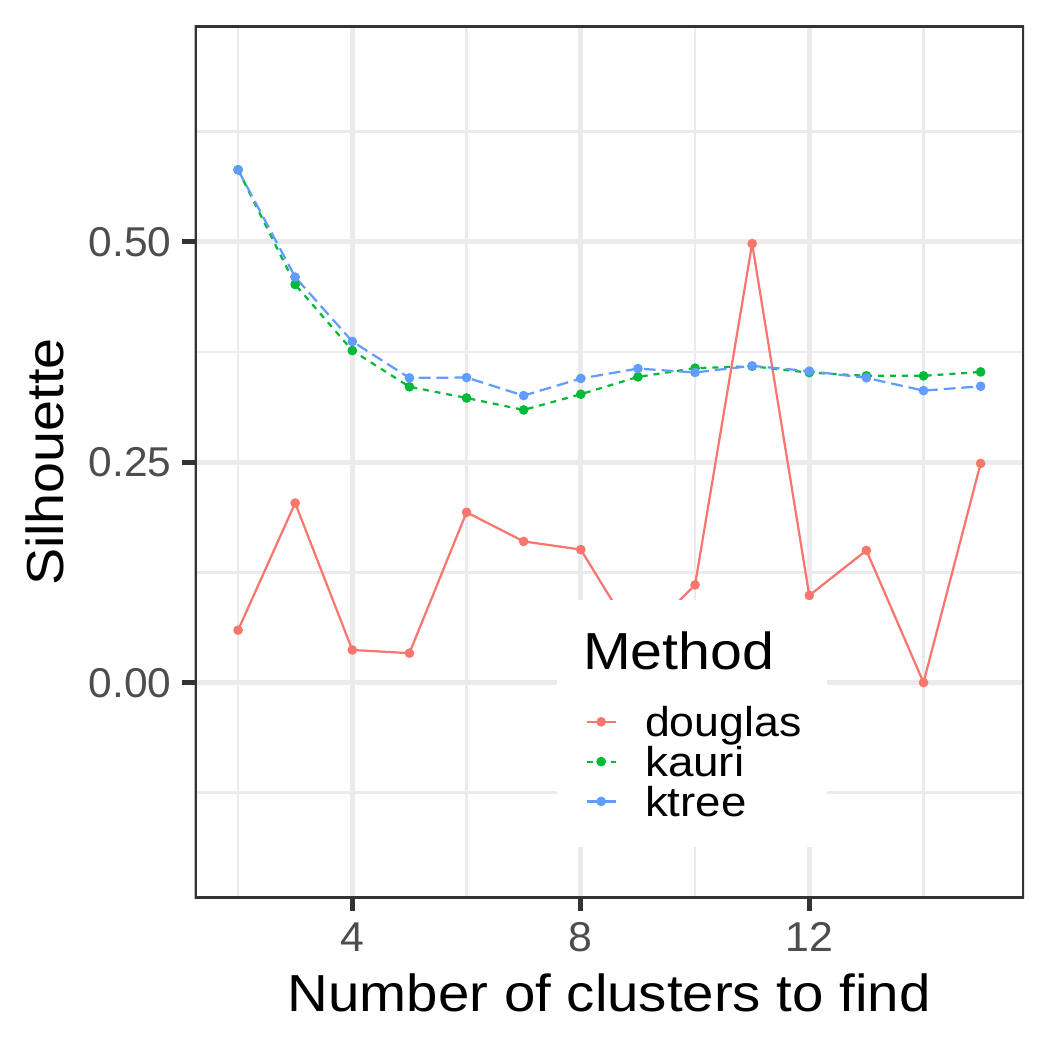}\label{sfig:iris_silhouette}}\hfil
    \subfloat[][Haberman's survival (3/3/2)]{\includegraphics[width=0.2\linewidth]{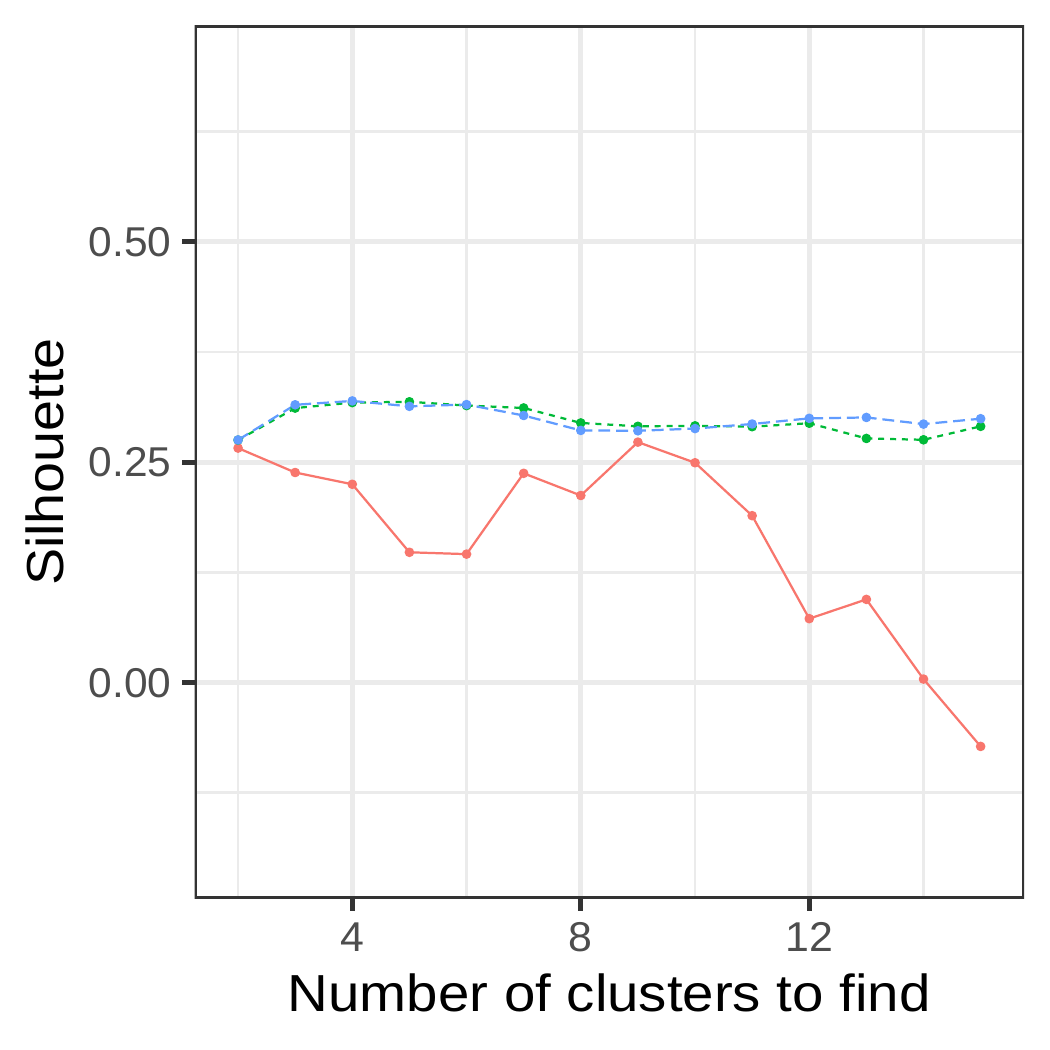}\label{sfig:haberman_silhouette}}\hfil
    \subfloat[][Breast cancer Wisconsin (2/2/4)]{\includegraphics[width=0.2\linewidth]{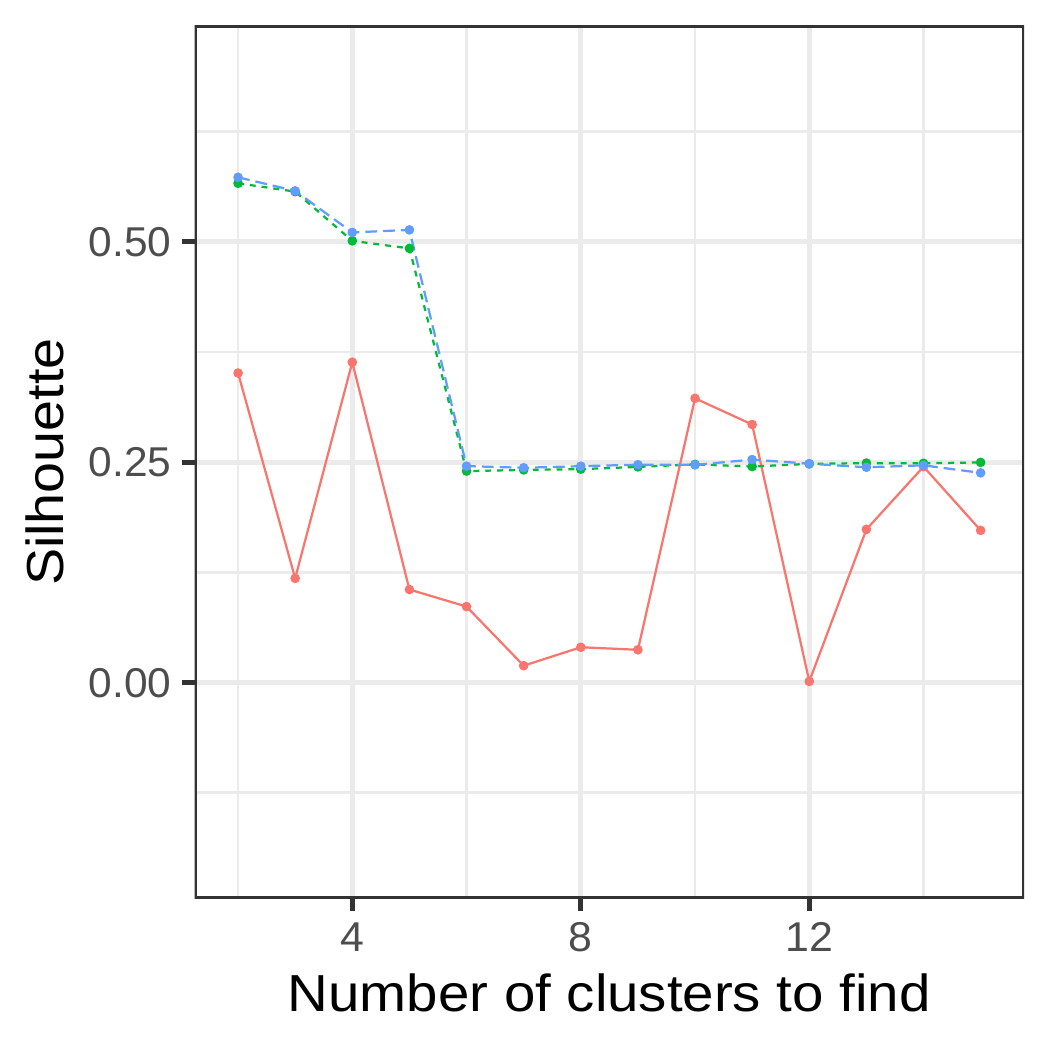}\label{sfig:breast_cancer_silhouette}}\hfil
    \subfloat[][Mice protein expression (13/13/13)]{\includegraphics[width=0.2\linewidth]{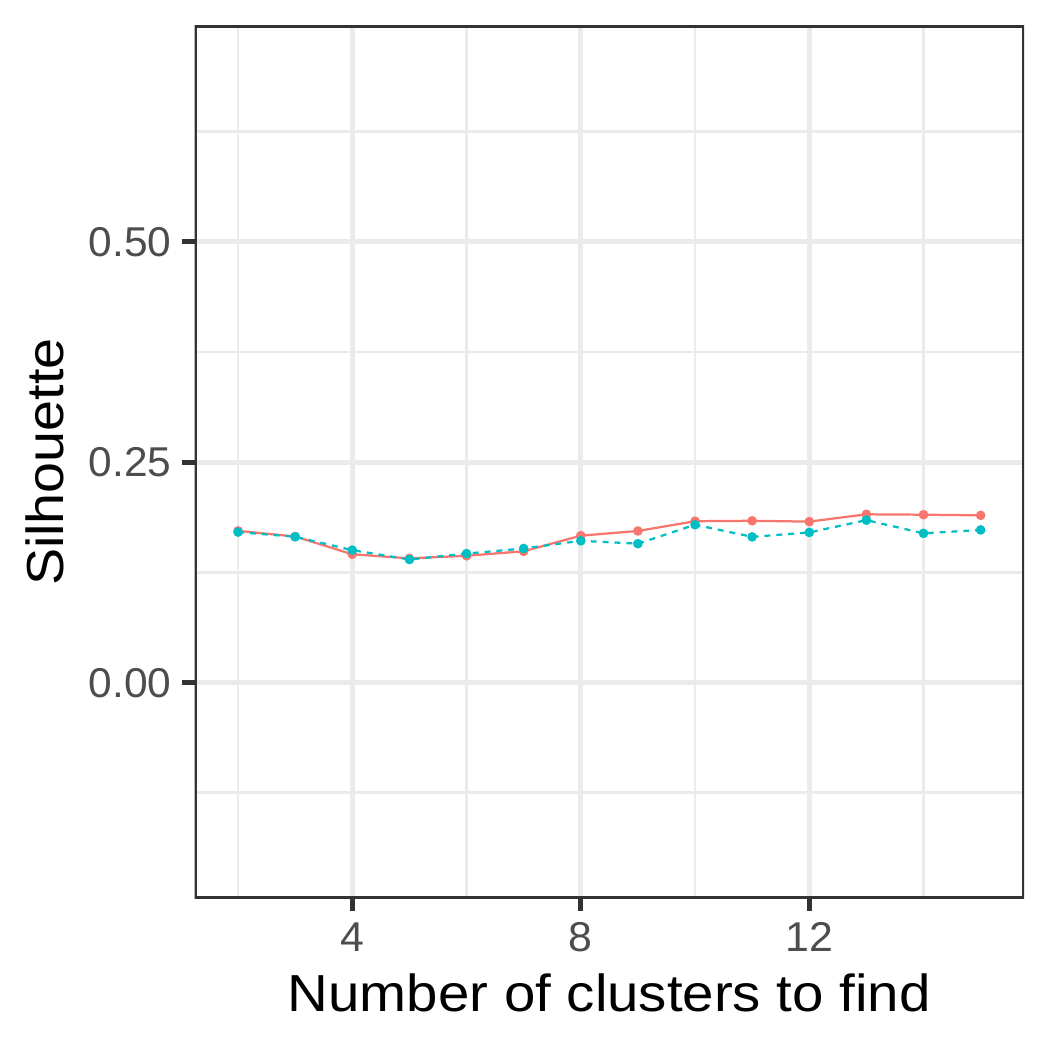}\label{sfig:mice_silhouette}}
    \caption{Silhouette scores of Kauri and Douglas for various numbers of clusters compared with the KMeans+Tree algorithm. Selected number of clusters are written in parentheses as (Kauri / KMeans+Tree / Douglas).}
    \label{fig:silhouette_scores}
\end{figure}
\begin{figure}
    \centering
    \subfloat[][Iris (?/?)]{\includegraphics[width=0.2\linewidth]{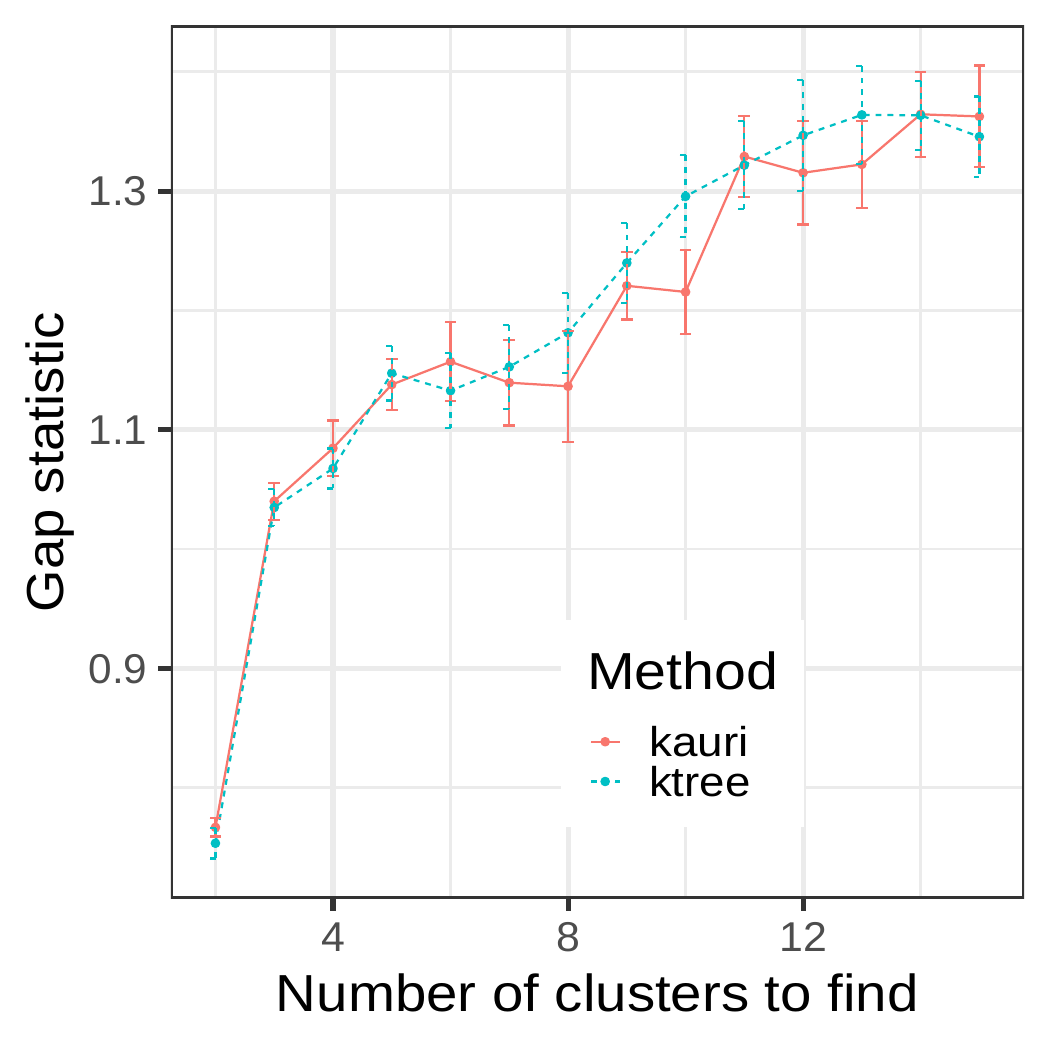}\label{sfig:iris_gap}}\hfil
    \subfloat[][Haberman's survival (5/4)]{\includegraphics[width=0.2\linewidth]{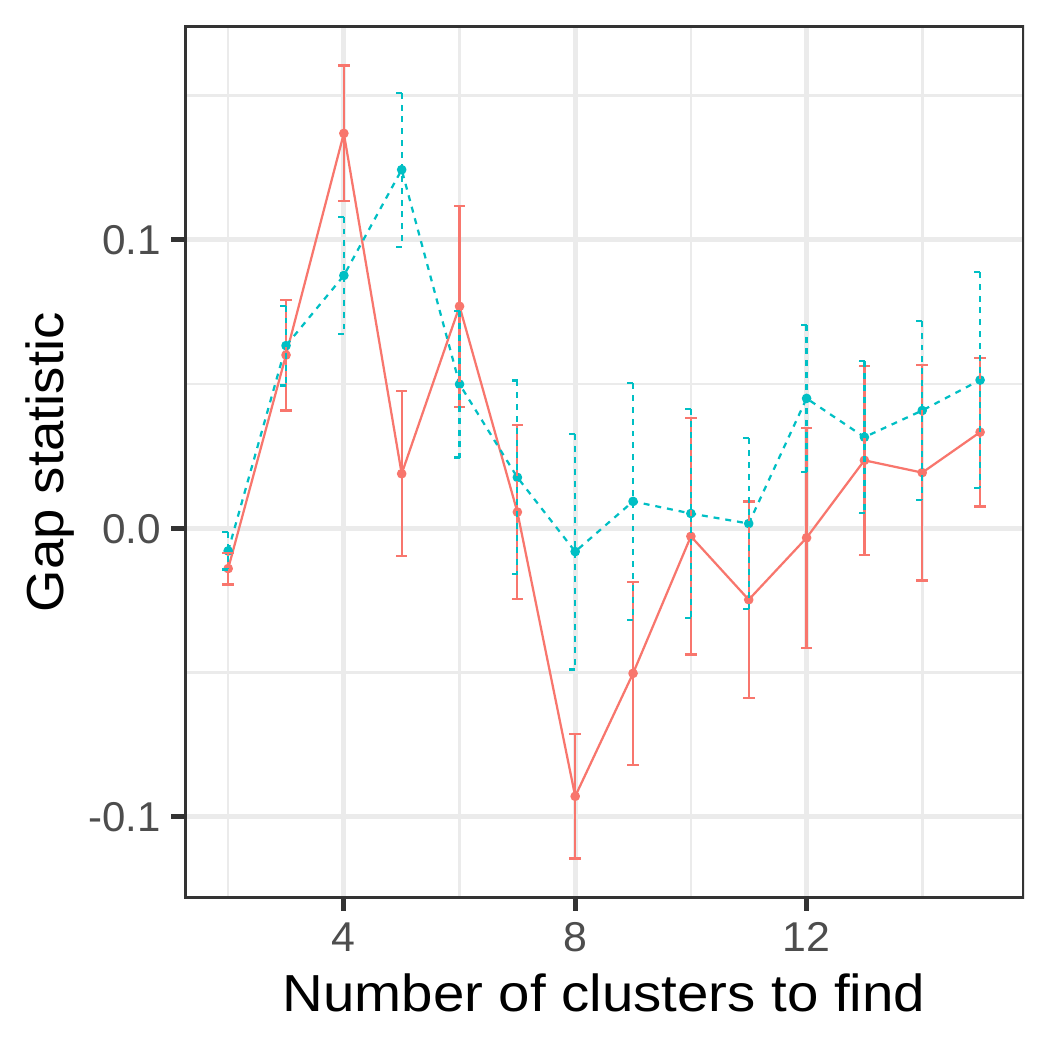}\label{sfig:haberman_gap}}\hfil
    \subfloat[][Breast cancer Wisconsin (?/?)]{\includegraphics[width=0.2\linewidth]{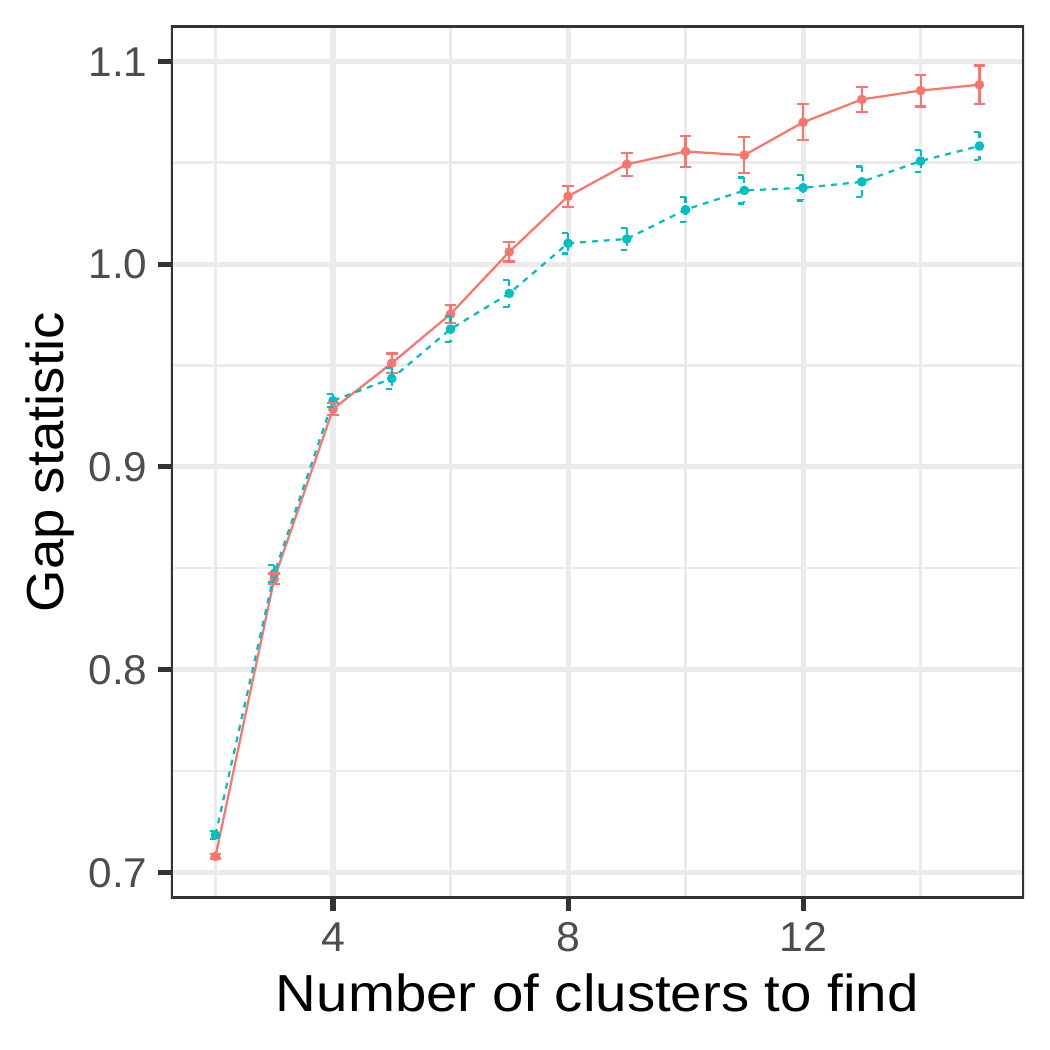}\label{sfig:breast_cancer_gap}}\hfil
    \subfloat[][Mice protein expression (?/?)]{\includegraphics[width=0.2\linewidth]{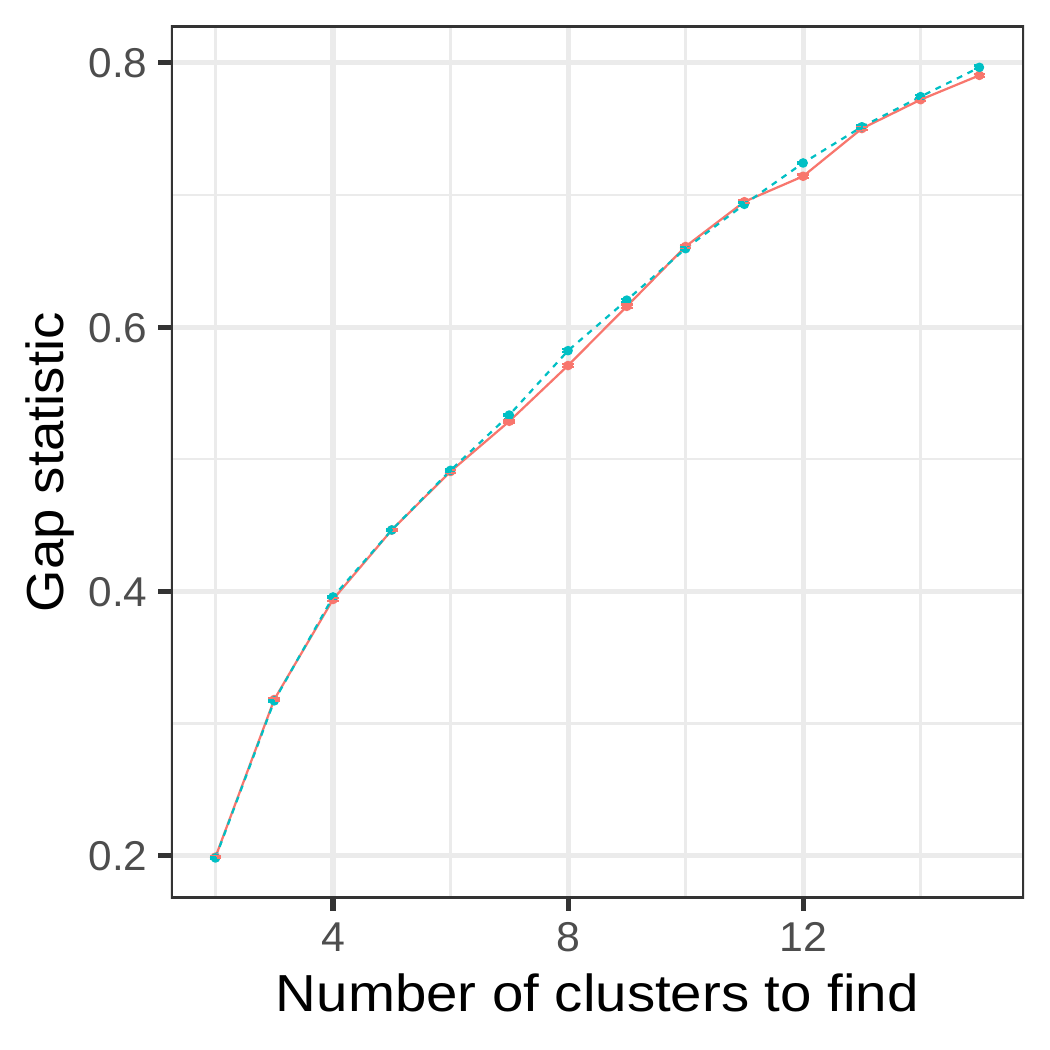}\label{sfig:mice_gap}}
    \caption{Gap statistic curves of Kauri various numbers of clusters compared with the KMeans+Tree algorithm. The selected number of clusters are written in parentheses as (Kauri / KMeans+Tree). We wrote ? when we were unable to determine a relevant gap within the limit of one standard deviation.}
    \label{fig:gap_scores}
\end{figure}

One subsidiary question remains the choice of the number of clusters. In the general context of discriminative clustering, we cannot benefit from common Bayesian tools such as the Bayesian information criterion~\cite{schwarz_estimating_1978} or the integrated complete likelihood~\cite{biernacki_assessing_2000} because we cannot define a likelihood. Common tools for model selection with KMeans are the elbow method, despite recent critics~\cite{frich_stop_2023}, the maximum silhouette score or the gap statistic~\cite{tibshirani_estimating_2001}. The maximum silhouette consists in seeking the number of clusters with low intra-cluster distance and high inter-cluster distance. The gap statistic consists in comparing the progressive decrease of a weighted sum of squares against a null hypothesis and selecting the number of clusters at which the gap suddenly decreases beyond standard deviation bounds. We ran these two methods as examples on four datasets and summarised the results in the figures~\ref{fig:silhouette_scores} and~\ref{fig:gap_scores}. We only computed the gap statistic for the Kauri method since running bootstrap estimates of the required weighted sum of squares for Douglas was too time-consuming. We compared the algorithms with the performances of the combination KMeans+Tree.

To compute the gap statistic in model selection~\cite{tibshirani_estimating_2001}, the central element to compute is the weighted sum of squares (WCSS) defined as:
\begin{equation}
    W_K = \sum_{k=1}^K \frac{1}{2 \card{\cluster_k}} \sum_{\x_i,\x_j \in \cluster_k} \norm{\x_i - \x_j}_2^2.
\end{equation}
A natural extension to compute this WCSS in the kernel KMeans is to switch from the usual Euclidean space to a Hilbert space $\mathcal{H}$. Then, we need to use the kernel trick to properly compute WCSS:
\begin{equation}
    W_K = \sum_{k=1}^K \frac{1}{2 \card{\cluster_k}} \sum_{\x_i,\x_j \in \cluster_k} \kappa(\x_i,\x_i) + \kappa(\x_j,\x_j) - 2 \kappa(\x_i,\x_j).
\end{equation}
However, that last equation is in fact equivalent to the subtraction of the data kernel and the objective function of Kauri as shown in the section~\ref{sssec:kernel_kmeans_relationship}. We deduce:
\begin{equation}
    W_K = \sigma(\dataset\times \dataset) - \objective.
\end{equation}
We can therefore use the gap statistic to select models with Kauri.

Our first main observation from both figures is that the Kauri algorithm follows very well the curves from the combination KMeans+Tree, therefore it seems reasonable to expect model selection methods to perform equally well with KMeans or Kauri in general. Our second observation is that apart from the mice protein dataset where all methods agreed with Silhouette scores to the same number of clusters (Fig.~\ref{sfig:mice_silhouette}), the number of clusters is often close or equal to the number of classes, except for Douglas on the iris dataset which Silhouette scores spiked at 11 clusters. However, the selection with the gap statistic was not as successful because we did not get any clear gap decrease apart from the Haberman's survival dataset (Fig.~\ref{sfig:haberman_gap}) where the number of clusters is far from the number of classes. This is as well a good reminder that the number of classes is not necessarily the optimal number of clusters, an ill-defined concept.
